# Supplementary material for: Fully parameter-free calculation of optical spectra for insulators, semiconductors and metals from a simple polarization functional
Source: arXiv:1503.00333 ancillary file (2015-06-10)
Supplement: Supplementary file 1 [file suppmat.pdf]

# Supplemental material for "Fully parameter-free calculation of optical spectra for insulators, semiconductors and metals from a simple polarization functional"

J. A. Berger[1]

[1] *Laboratoire de Chimie et Physique Quantiques, IRSAMC, Université Toulouse III - Paul Sabatier, CNRS and European Theoretical Spectroscopy Facility (ETSF), 118 Route de Narbonne, 31062 Toulouse Cedex, France*

## EXACT CONSTRAINT FOR BOUND EXCITONS

In this section we derive Eq. (11) of the article following similar arguments as in Ref. [1]. We can rewrite Eq. (10) of the article, with $\overleftrightarrow{\chi}_e^0 = \overleftrightarrow{\chi}_e^{RPA}$, according to

$$\chi_e(\omega) = \frac{\chi_e^{RPA}(\omega)}{1 - \chi_e^{RPA}(\omega)\alpha(\omega)}, \tag{1}$$

where for simplicity we assume that $\overleftrightarrow{\chi}_e(\omega)$, $\overleftrightarrow{\chi}_e^{RPA}(\omega)$ and $\overleftrightarrow{\alpha}(\omega)$ are isotropic, *i.e.*, $\alpha_{ij}(\omega) = \alpha(\omega)\delta_{ij}$, etc..

To observe a bound exciton, $\text{Im}[\chi_e(\omega)]$ has to be nonzero below the band gap. From the above equation we learn that for energies below the gap, where $\text{Im}[\chi_e^{RPA}(\omega)] = 0$, we have

$$\text{Im}[\chi_e(\omega)] = \text{Re}[\chi_e^{RPA}(\omega)]\text{Im}\left[\frac{1}{1 - \chi_e^{RPA}(\omega)\alpha(\omega)}\right] = \tag{2}$$

$$\frac{(\text{Re}[\chi_e^{RPA}(\omega)])^2\text{Im}[\alpha(\omega)]}{(1 - \text{Re}[\chi_e^{RPA}(\omega)]\text{Re}[\alpha(\omega)])^2 + (\text{Re}[\chi_e^{RPA}(\omega)]\text{Im}[\alpha(\omega)])^2}. \tag{3}$$

From Eq. (3) we see that a bound exciton can only be obtained if for some frequency $\omega = \omega_{be}$ below the band gap, we have

$$\text{Re}[\alpha(\omega_{be})] = \frac{1}{\text{Re}[\chi_e^{RPA}(\omega_{be})]}, \tag{4}$$

and $\text{Im}[\alpha(\omega_{be})]$ vanishes or is small. The corresponding value of $\text{Im}[\chi_e(\omega)]$ is then given by

$$\text{Im}[\chi_e(\omega_{be})] = \frac{\text{Re}[\chi_e^{RPA}(\omega_{be})]}{\text{Im}[\alpha(\omega_{be})]}. \tag{5}$$

Equation (4) corresponds to Eq. (11) of the article.

## DERIVATION OF THE STATIC KERNEL

In this section we derive Eq. (12) of the article. To apply Eq. (4) in calculations requires the knowledge of $\omega_{be}$ which is unknown. Therefore, we would like to rewrite this equation in terms of known quantities. Here we will derive such an expression by considering the limiting case of a low-density insulator, *i.e.*, an insulator for which the density $N_e/V$ is small, where $N_e$ is the number of electrons in the unit cell and $V$ is the volume of the unit cell. Such an insulator typically has a large band gap, a small dielectric constant and an optical spectrum that is dominated by a sharp bound exciton.

In the RPA optical spectrum the bound exciton is absent and there will be absorption only in the energy range given by the interband transitions. Therefore we can describe the RPA susceptibility with the following Lorentz model [2],

$$\chi_e^{RPA}(\omega) \approx -\frac{\omega_p^2}{8\pi\omega_{ar}}\left[\frac{1}{\omega - \omega_{ar} + i\gamma} - \frac{1}{\omega + \omega_{ar} + i\gamma}\right], \tag{6}$$

where $\omega_{ar}$ is the average resonance frequency and $\gamma$ determines the finite width of $\omega_{ar}$. The prefactor $-\omega_p^2/(8\pi\omega_{ar})$ ensures that the f-sum rule given by

$$\int_0^\infty d\omega\omega\text{Im}\chi_e(\omega) = \frac{\omega_p^2}{8}, \tag{7}$$

is satisfied. Here $\omega_p = \sqrt{4\pi N_e/V}$ is the plasma frequency. It was shown analytically that in the limit $V \to \infty$ the RPA loss function (in the long-wavelength limit) and the RPA optical spectrum become identical [3]. The RPA loss function is centered around $\omega = \omega_p$. Therefore, for a low-density insulator we have that $\omega_{ar} \approx \omega_p$ and we can rewrite Eq. (6) as

$$\chi_e^{RPA}(\omega) \approx -\frac{\omega_p}{8\pi}\left[\frac{1}{\omega - \omega_p + i\gamma} - \frac{1}{\omega + \omega_p + i\gamma}\right]. \tag{8}$$

Since we want to get an estimate of $\chi_e^{RPA}(\omega_{be})$, the main features of $\chi_e^{RPA}(\omega)$ that this model should capture is its behavior below the band gap. In this region $\chi_e^{RPA}(\omega)$ is purely real and a smooth, monotonous function of the frequency.

The true absorption spectrum is dominated by a sharp bound exciton at $\omega = \omega_{be}$. Therefore, $\chi_e(\omega)$ can be described according to the following Lorentz model,

$$\chi_e(\omega) \approx -\frac{\omega_{be}}{8\pi}\left[\frac{1}{\omega - \omega_{be} + i\eta} - \frac{1}{\omega + \omega_{be} + i\eta}\right]. \tag{9}$$

where $\eta \simeq 0$ determines the width of the bound exciton and the prefactor $-\omega_{be}/(8\pi)$ ensures that $\epsilon_M(0) = \epsilon_M^{RPA}(0)$, since $\epsilon_M^{RPA}(0)$ is a good approximation to $\epsilon_M(0)$. This is more realistic than to ensure the f-sum rule since the model for $\chi_e(\omega)$ describes the main part of the spectrum, *i.e.*, the bound exciton, but not the whole spectrum as was the case for $\chi^{RPA}(\omega)$.

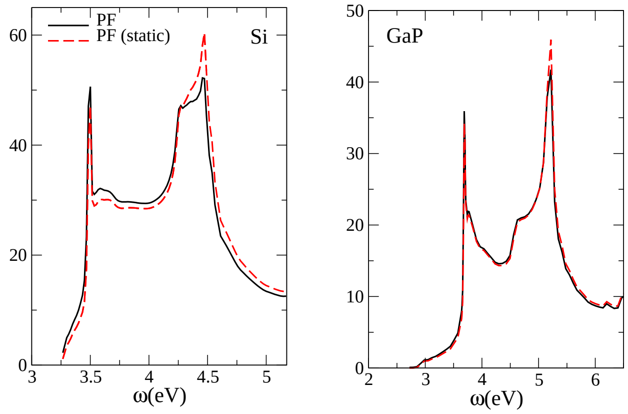


FIG. 1. (Color online) The optical absorption spectra of bulk silicon and GaP. Solid line (black): polarization functional (PF); Dashed line (red): polarization functional with only its static part.

A relation between $\omega_{be}$ and $\omega_p$ can be found by using the fact that $\omega_p$ corresponds approximately to the frequency at which $\mathrm{Re}[\epsilon_M(\omega)] = 0$ and $\mathrm{Im}[\epsilon_M(\omega)] \ll 1$. Solving the equation

$$\mathrm{Re}[\epsilon_M(\omega_p)] = 1 + 4\pi \mathrm{Re}[\chi_e(\omega_p)] = 0 \tag{10}$$

leads to the relation

$$\omega_p = \sqrt{2}\omega_{be}. \tag{11}$$

As mentioned before, below the band gap $\chi_e^{RPA}(\omega)$ is purely real and a smooth, monotonous function of the frequency. We can therefore expand it as a Taylor series around $\omega = 0$ and evaluate the series at $\omega = \omega_{be}$. We obtain

$$\chi_e^{RPA}(\omega_{be}) = \sum_{n=0}^{\infty} \frac{\omega_{be}^n}{n!} \left. \frac{d^n \chi_e^{RPA}(\omega)}{d\omega^n} \right|_{\omega=0} \tag{12}$$

$$= \chi_e^{RPA}(0) + 4\pi \sum_{n=1}^{\infty} \left[\frac{1}{2}\right]^n [\chi_e^{RPA}(0)]^2 \tag{13}$$

$$= \chi_e^{RPA}(0) + 4\pi[\chi_e^{RPA}(0)]^2 \tag{14}$$

where in the second step we used Eq. (11) and the fact that $\gamma^2 \ll \omega_p^2$. Since $\epsilon_M^{RPA}(\omega) = 1 + 4\pi\chi_e^{RPA}(\omega)$ we finally obtain

$$\chi_e^{RPA}(\omega_{be}) = \chi_e^{RPA}(0)\epsilon_M^{RPA}(0). \tag{15}$$

Substitution of this expression into Eq. (4) then leads to the following static $\alpha$,

$$\alpha \equiv \mathrm{Re}[\alpha(\omega_{be})] = \frac{1}{\chi_e^{RPA}(0)\epsilon_M^{RPA}(0)}. \tag{16}$$

This is Eq. (12) of the article.

## COMPARISON OF THE STATIC AND DYNAMICAL POLARIZATION FUNCTIONAL FOR SEMICONDUCTORS

In this section we show that the static polarization functional given in Eq. (12) of the article leads to optical spectra for semiconductors that are similar to those obtained with the fully dynamical polarization functional given in Eq. (14) of the article. In Fig. 1 we report the optical spectra of bulk silicon and GaP using the static and dynamical functionals. We see that the differences are indeed small. We note that, instead, the dynamical part is crucial to obtain the finite width of bound excitons and Drude tails in insulators and metals, respectively.


[1] F. Sottile, K. Karlsson, L. Reining, and F. Aryasetiawan, Phys. Rev. B **68**, 205112 (2003).

[2] S. Botti, A. Fourreau, F. Nguyen, Y.-O. Renault, F. Sottile, and L. Reining, Phys. Rev. B **72**, 125203 (2005).

[3] F. Sottile, F. Bruneval, A. G. Marinopoulos, L. K. Dash, S. Botti, V. Olevano, N. Vast, A. Rubio, and L. Reining, Int. J. Quantum Chem. **102**, 684 (2005).
